# Supplementary material for: Towards a unified language in experimental designs propagated by a software framework
Source: arXiv:2307.11593 ancillary file (2023-07-24)
Supplement: Supplementary file 1 [file supp.pdf]

# Supplmentary material for “Towards a unified language in experimental designs propagated by a software framework”

Emi Tanaka

2023-07-24

## Applications

The following code uses the R-package `edibble` (Tanaka 2023) in the R language (R Core Team 2020) to construct three types of experimental design described in the main paper. The full design tables for the split-plot design, complex nested design and unbalanced factorial design are shown in Table 1, Table 2 and Table 3, respectively.

```
library(edibble)
```

## Classic Split-Plot Design

The experiment, described in Fisher (1950), is a classic split-plot design for testing the yield of a crop with 12 varieties under 3 different types of fertilizer.

Below we define the unit and treatment factors.

```
des1str <- design("Fisher's split-plot design") %>%  
  set_units(patch = 36,  
            plot = nested_in(patch, 3)) %>%  
  set_trts(variety = 12,  
           fertilizer = c("basal", "sulphate", "chloride"))
```

You may also set the responses.

```
des1strr <- des1str %>%
  set_rcrds(yield = plot,
            biomass = patch)
```

At this stage, the design is not complete and stored in the network form.

```
des1strr
```

Fisher's split-plot design

```
+--patch (36 levels)
| +-plot (108 levels)
| | \-yield
| | \-biomass
+-variety (12 levels)
\-fertilizer (3 levels)
```

We need to specify the relationship between factors. We can then get the design table.

```
des1 <- des1strr %>%
  allot_trts(variety ~ patch,
             fertilizer ~ plot) %>%
  assign_trts(seed = 1,
              order = c("random", "random")) %>%
  serve_table()
```

The output is a special class of `data.frame`. See Table 1 for the full design table.

```
des1
```

```
# Fisher's split-plot design
# An edibble: 108 x 6
```

|   | patch      | plot        | variety   | fertilizer | yield  | biomass |
|---|------------|-------------|-----------|------------|--------|---------|
|   | <unit(36)> | <unit(108)> | <trt(12)> | <trt(3)>   | <rcrd> | <rcrd>  |
| 1 | patch1     | plot1       | variety11 | sulphate   | o      | o       |
| 2 | patch1     | plot2       | variety11 | chloride   | o      | x       |
| 3 | patch1     | plot3       | variety11 | basal      | o      | x       |
| 4 | patch2     | plot4       | variety9  | chloride   | o      | o       |
| 5 | patch2     | plot5       | variety9  | sulphate   | o      | x       |
| 6 | patch2     | plot6       | variety9  | basal      | o      | x       |
| 7 | patch3     | plot7       | variety6  | sulphate   | o      | o       |
| 8 | patch3     | plot8       | variety6  | basal      | o      | x       |

```

9      patch3      plot9 variety6      chloride      o      x
10     patch4      plot10 variety2      basal      o      o
# i 98 more rows

```

Table 1: Design table output for the classic split plot design.

| patch   | plot   | variety   | fertilizer | yield | biomass |
|---------|--------|-----------|------------|-------|---------|
| patch1  | plot1  | variety11 | sulphate   | NA    | NA      |
| patch1  | plot2  | variety11 | chloride   | NA    | NA      |
| patch1  | plot3  | variety11 | basal      | NA    | NA      |
| patch2  | plot4  | variety9  | chloride   | NA    | NA      |
| patch2  | plot5  | variety9  | sulphate   | NA    | NA      |
| patch2  | plot6  | variety9  | basal      | NA    | NA      |
| patch3  | plot7  | variety6  | sulphate   | NA    | NA      |
| patch3  | plot8  | variety6  | basal      | NA    | NA      |
| patch3  | plot9  | variety6  | chloride   | NA    | NA      |
| patch4  | plot10 | variety2  | basal      | NA    | NA      |
| patch4  | plot11 | variety2  | chloride   | NA    | NA      |
| patch4  | plot12 | variety2  | sulphate   | NA    | NA      |
| patch5  | plot13 | variety5  | basal      | NA    | NA      |
| patch5  | plot14 | variety5  | chloride   | NA    | NA      |
| patch5  | plot15 | variety5  | sulphate   | NA    | NA      |
| patch6  | plot16 | variety5  | sulphate   | NA    | NA      |
| patch6  | plot17 | variety5  | chloride   | NA    | NA      |
| patch6  | plot18 | variety5  | basal      | NA    | NA      |
| patch7  | plot19 | variety8  | basal      | NA    | NA      |
| patch7  | plot20 | variety8  | sulphate   | NA    | NA      |
| patch7  | plot21 | variety8  | chloride   | NA    | NA      |
| patch8  | plot22 | variety10 | chloride   | NA    | NA      |
| patch8  | plot23 | variety10 | sulphate   | NA    | NA      |
| patch8  | plot24 | variety10 | basal      | NA    | NA      |
| patch9  | plot25 | variety1  | basal      | NA    | NA      |
| patch9  | plot26 | variety1  | sulphate   | NA    | NA      |
| patch9  | plot27 | variety1  | chloride   | NA    | NA      |
| patch10 | plot28 | variety3  | chloride   | NA    | NA      |
| patch10 | plot29 | variety3  | sulphate   | NA    | NA      |
| patch10 | plot30 | variety3  | basal      | NA    | NA      |
| patch11 | plot31 | variety3  | chloride   | NA    | NA      |
| patch11 | plot32 | variety3  | basal      | NA    | NA      |
| patch11 | plot33 | variety3  | sulphate   | NA    | NA      |
| patch12 | plot34 | variety8  | basal      | NA    | NA      |
| patch12 | plot35 | variety8  | sulphate   | NA    | NA      |

| patch   | plot   | variety   | fertilizer | yield | biomass |
|---------|--------|-----------|------------|-------|---------|
| patch12 | plot36 | variety8  | chloride   | NA    | NA      |
| patch13 | plot37 | variety3  | chloride   | NA    | NA      |
| patch13 | plot38 | variety3  | sulphate   | NA    | NA      |
| patch13 | plot39 | variety3  | basal      | NA    | NA      |
| patch14 | plot40 | variety12 | basal      | NA    | NA      |
| patch14 | plot41 | variety12 | sulphate   | NA    | NA      |
| patch14 | plot42 | variety12 | chloride   | NA    | NA      |
| patch15 | plot43 | variety11 | basal      | NA    | NA      |
| patch15 | plot44 | variety11 | sulphate   | NA    | NA      |
| patch15 | plot45 | variety11 | chloride   | NA    | NA      |
| patch16 | plot46 | variety12 | sulphate   | NA    | NA      |
| patch16 | plot47 | variety12 | chloride   | NA    | NA      |
| patch16 | plot48 | variety12 | basal      | NA    | NA      |
| patch17 | plot49 | variety10 | basal      | NA    | NA      |
| patch17 | plot50 | variety10 | chloride   | NA    | NA      |
| patch17 | plot51 | variety10 | sulphate   | NA    | NA      |
| patch18 | plot52 | variety4  | basal      | NA    | NA      |
| patch18 | plot53 | variety4  | chloride   | NA    | NA      |
| patch18 | plot54 | variety4  | sulphate   | NA    | NA      |
| patch19 | plot55 | variety5  | basal      | NA    | NA      |
| patch19 | plot56 | variety5  | chloride   | NA    | NA      |
| patch19 | plot57 | variety5  | sulphate   | NA    | NA      |
| patch20 | plot58 | variety11 | basal      | NA    | NA      |
| patch20 | plot59 | variety11 | chloride   | NA    | NA      |
| patch20 | plot60 | variety11 | sulphate   | NA    | NA      |
| patch21 | plot61 | variety8  | chloride   | NA    | NA      |
| patch21 | plot62 | variety8  | sulphate   | NA    | NA      |
| patch21 | plot63 | variety8  | basal      | NA    | NA      |
| patch22 | plot64 | variety9  | sulphate   | NA    | NA      |
| patch22 | plot65 | variety9  | chloride   | NA    | NA      |
| patch22 | plot66 | variety9  | basal      | NA    | NA      |
| patch23 | plot67 | variety7  | basal      | NA    | NA      |
| patch23 | plot68 | variety7  | chloride   | NA    | NA      |
| patch23 | plot69 | variety7  | sulphate   | NA    | NA      |
| patch24 | plot70 | variety1  | chloride   | NA    | NA      |
| patch24 | plot71 | variety1  | basal      | NA    | NA      |
| patch24 | plot72 | variety1  | sulphate   | NA    | NA      |
| patch25 | plot73 | variety7  | basal      | NA    | NA      |
| patch25 | plot74 | variety7  | chloride   | NA    | NA      |
| patch25 | plot75 | variety7  | sulphate   | NA    | NA      |
| patch26 | plot76 | variety7  | chloride   | NA    | NA      |

| patch   | plot    | variety   | fertilizer | yield | biomass |
|---------|---------|-----------|------------|-------|---------|
| patch26 | plot77  | variety7  | basal      | NA    | NA      |
| patch26 | plot78  | variety7  | sulphate   | NA    | NA      |
| patch27 | plot79  | variety2  | basal      | NA    | NA      |
| patch27 | plot80  | variety2  | chloride   | NA    | NA      |
| patch27 | plot81  | variety2  | sulphate   | NA    | NA      |
| patch28 | plot82  | variety12 | basal      | NA    | NA      |
| patch28 | plot83  | variety12 | chloride   | NA    | NA      |
| patch28 | plot84  | variety12 | sulphate   | NA    | NA      |
| patch29 | plot85  | variety4  | basal      | NA    | NA      |
| patch29 | plot86  | variety4  | sulphate   | NA    | NA      |
| patch29 | plot87  | variety4  | chloride   | NA    | NA      |
| patch30 | plot88  | variety4  | chloride   | NA    | NA      |
| patch30 | plot89  | variety4  | basal      | NA    | NA      |
| patch30 | plot90  | variety4  | sulphate   | NA    | NA      |
| patch31 | plot91  | variety9  | sulphate   | NA    | NA      |
| patch31 | plot92  | variety9  | basal      | NA    | NA      |
| patch31 | plot93  | variety9  | chloride   | NA    | NA      |
| patch32 | plot94  | variety6  | chloride   | NA    | NA      |
| patch32 | plot95  | variety6  | sulphate   | NA    | NA      |
| patch32 | plot96  | variety6  | basal      | NA    | NA      |
| patch33 | plot97  | variety1  | sulphate   | NA    | NA      |
| patch33 | plot98  | variety1  | chloride   | NA    | NA      |
| patch33 | plot99  | variety1  | basal      | NA    | NA      |
| patch34 | plot100 | variety2  | basal      | NA    | NA      |
| patch34 | plot101 | variety2  | chloride   | NA    | NA      |
| patch34 | plot102 | variety2  | sulphate   | NA    | NA      |
| patch35 | plot103 | variety10 | sulphate   | NA    | NA      |
| patch35 | plot104 | variety10 | basal      | NA    | NA      |
| patch35 | plot105 | variety10 | chloride   | NA    | NA      |
| patch36 | plot106 | variety6  | sulphate   | NA    | NA      |
| patch36 | plot107 | variety6  | chloride   | NA    | NA      |
| patch36 | plot108 | variety6  | basal      | NA    | NA      |

### Alternative unit specification

In the above code, we have specified the units as below.

```
des1unit <- design("Unit specification") %>%
  set_units(patch = 36,
```

```
plot = nested_in(patch, 3))
```

In another instance, you may be told the total number of plots ( $36 \times 3 = 108$ ). In this case, it may cognitively make more sense to specify the total number of plots directly as below.

```
des1unitalt <- design("Alternative unit specification") %>%  
  set_units(patch = 36,  
            plot = 108)
```

The above code does not, however, the relationship between `patch` and `plot`. For this, we can use `allot_units()` to signal the nesting of the units and `assign_units()` to actually assign the small units to large units as below.

```
des1unitalt %>%  
  allot_units(patch ~ plot) %>%  
  assign_units("systematic")
```

```
Alternative unit specification  
\-patch (36 levels)  
  \-plot (108 levels)  
Allotment:
```

The above is more verbose than the first approach, however, this may cognitively align with how the units are specified in conversation. Ultimately, it will be user choice on how this is specified, but the end result is essentially the same.

## Complex Nested Design

Consider next the experiment in Martin, Johnson, and Forsyth (1996) aimed to investigate if insecticides used to control grasshoppers affected the weight of young chicks of ring-necked pheasants, either by affecting the grass around the chicks or by affecting the grasshoppers eaten by the chicks.

```
1 des2 <- design("Complex nested factorial design") %>%  
2   set_trts(insecticide = 3,  
3           dose_level  = c("low", "high"),  
4           food_type   = c("sprayed", "unsprayed")) %>%  
5   set_units(week = 3,  
6           strip = nested_in(week, 3),  
7           swath = nested_in(strip, 2),
```

```

8         pen    = nested_in(swath, 2),
9         chick = nested_in(pen, 6)) %>%
10     allot_trts(insecticide ~ strip,
11               dose_level ~ swath,
12               food_type ~ pen) %>%
13     assign_trts(seed = 1) %>%
14     serve_table()

```

Table 2: Design table output for the complex nested design.

| insecticide  | dose_level | food_type | week  | strip  | swath  | pen  | chick   |
|--------------|------------|-----------|-------|--------|--------|------|---------|
| insecticide2 | high       | unsprayed | week1 | strip1 | swath1 | pen1 | chick1  |
| insecticide2 | high       | unsprayed | week1 | strip1 | swath1 | pen1 | chick2  |
| insecticide2 | high       | unsprayed | week1 | strip1 | swath1 | pen1 | chick3  |
| insecticide2 | high       | unsprayed | week1 | strip1 | swath1 | pen1 | chick4  |
| insecticide2 | high       | unsprayed | week1 | strip1 | swath1 | pen1 | chick5  |
| insecticide2 | high       | unsprayed | week1 | strip1 | swath1 | pen1 | chick6  |
| insecticide2 | high       | sprayed   | week1 | strip1 | swath1 | pen2 | chick7  |
| insecticide2 | high       | sprayed   | week1 | strip1 | swath1 | pen2 | chick8  |
| insecticide2 | high       | sprayed   | week1 | strip1 | swath1 | pen2 | chick9  |
| insecticide2 | high       | sprayed   | week1 | strip1 | swath1 | pen2 | chick10 |
| insecticide2 | high       | sprayed   | week1 | strip1 | swath1 | pen2 | chick11 |
| insecticide2 | high       | sprayed   | week1 | strip1 | swath1 | pen2 | chick12 |
| insecticide2 | low        | unsprayed | week1 | strip1 | swath2 | pen3 | chick13 |
| insecticide2 | low        | unsprayed | week1 | strip1 | swath2 | pen3 | chick14 |
| insecticide2 | low        | unsprayed | week1 | strip1 | swath2 | pen3 | chick15 |
| insecticide2 | low        | unsprayed | week1 | strip1 | swath2 | pen3 | chick16 |
| insecticide2 | low        | unsprayed | week1 | strip1 | swath2 | pen3 | chick17 |
| insecticide2 | low        | unsprayed | week1 | strip1 | swath2 | pen3 | chick18 |
| insecticide2 | low        | sprayed   | week1 | strip1 | swath2 | pen4 | chick19 |
| insecticide2 | low        | sprayed   | week1 | strip1 | swath2 | pen4 | chick20 |
| insecticide2 | low        | sprayed   | week1 | strip1 | swath2 | pen4 | chick21 |
| insecticide2 | low        | sprayed   | week1 | strip1 | swath2 | pen4 | chick22 |
| insecticide2 | low        | sprayed   | week1 | strip1 | swath2 | pen4 | chick23 |
| insecticide2 | low        | sprayed   | week1 | strip1 | swath2 | pen4 | chick24 |
| insecticide3 | high       | sprayed   | week1 | strip2 | swath3 | pen5 | chick25 |
| insecticide3 | high       | sprayed   | week1 | strip2 | swath3 | pen5 | chick26 |
| insecticide3 | high       | sprayed   | week1 | strip2 | swath3 | pen5 | chick27 |
| insecticide3 | high       | sprayed   | week1 | strip2 | swath3 | pen5 | chick28 |
| insecticide3 | high       | sprayed   | week1 | strip2 | swath3 | pen5 | chick29 |
| insecticide3 | high       | sprayed   | week1 | strip2 | swath3 | pen5 | chick30 |

| insecticide  | dose_level | food_type | week  | strip  | swath  | pen   | chick   |
|--------------|------------|-----------|-------|--------|--------|-------|---------|
| insecticide3 | high       | unsprayed | week1 | strip2 | swath3 | pen6  | chick31 |
| insecticide3 | high       | unsprayed | week1 | strip2 | swath3 | pen6  | chick32 |
| insecticide3 | high       | unsprayed | week1 | strip2 | swath3 | pen6  | chick33 |
| insecticide3 | high       | unsprayed | week1 | strip2 | swath3 | pen6  | chick34 |
| insecticide3 | high       | unsprayed | week1 | strip2 | swath3 | pen6  | chick35 |
| insecticide3 | high       | unsprayed | week1 | strip2 | swath3 | pen6  | chick36 |
| insecticide3 | low        | unsprayed | week1 | strip2 | swath4 | pen7  | chick37 |
| insecticide3 | low        | unsprayed | week1 | strip2 | swath4 | pen7  | chick38 |
| insecticide3 | low        | unsprayed | week1 | strip2 | swath4 | pen7  | chick39 |
| insecticide3 | low        | unsprayed | week1 | strip2 | swath4 | pen7  | chick40 |
| insecticide3 | low        | unsprayed | week1 | strip2 | swath4 | pen7  | chick41 |
| insecticide3 | low        | unsprayed | week1 | strip2 | swath4 | pen7  | chick42 |
| insecticide3 | low        | sprayed   | week1 | strip2 | swath4 | pen8  | chick43 |
| insecticide3 | low        | sprayed   | week1 | strip2 | swath4 | pen8  | chick44 |
| insecticide3 | low        | sprayed   | week1 | strip2 | swath4 | pen8  | chick45 |
| insecticide3 | low        | sprayed   | week1 | strip2 | swath4 | pen8  | chick46 |
| insecticide3 | low        | sprayed   | week1 | strip2 | swath4 | pen8  | chick47 |
| insecticide3 | low        | sprayed   | week1 | strip2 | swath4 | pen8  | chick48 |
| insecticide1 | high       | sprayed   | week1 | strip3 | swath5 | pen9  | chick49 |
| insecticide1 | high       | sprayed   | week1 | strip3 | swath5 | pen9  | chick50 |
| insecticide1 | high       | sprayed   | week1 | strip3 | swath5 | pen9  | chick51 |
| insecticide1 | high       | sprayed   | week1 | strip3 | swath5 | pen9  | chick52 |
| insecticide1 | high       | sprayed   | week1 | strip3 | swath5 | pen9  | chick53 |
| insecticide1 | high       | sprayed   | week1 | strip3 | swath5 | pen9  | chick54 |
| insecticide1 | high       | unsprayed | week1 | strip3 | swath5 | pen10 | chick55 |
| insecticide1 | high       | unsprayed | week1 | strip3 | swath5 | pen10 | chick56 |
| insecticide1 | high       | unsprayed | week1 | strip3 | swath5 | pen10 | chick57 |
| insecticide1 | high       | unsprayed | week1 | strip3 | swath5 | pen10 | chick58 |
| insecticide1 | high       | unsprayed | week1 | strip3 | swath5 | pen10 | chick59 |
| insecticide1 | high       | unsprayed | week1 | strip3 | swath5 | pen10 | chick60 |
| insecticide1 | low        | unsprayed | week1 | strip3 | swath6 | pen11 | chick61 |
| insecticide1 | low        | unsprayed | week1 | strip3 | swath6 | pen11 | chick62 |
| insecticide1 | low        | unsprayed | week1 | strip3 | swath6 | pen11 | chick63 |
| insecticide1 | low        | unsprayed | week1 | strip3 | swath6 | pen11 | chick64 |
| insecticide1 | low        | unsprayed | week1 | strip3 | swath6 | pen11 | chick65 |
| insecticide1 | low        | unsprayed | week1 | strip3 | swath6 | pen11 | chick66 |
| insecticide1 | low        | sprayed   | week1 | strip3 | swath6 | pen12 | chick67 |
| insecticide1 | low        | sprayed   | week1 | strip3 | swath6 | pen12 | chick68 |
| insecticide1 | low        | sprayed   | week1 | strip3 | swath6 | pen12 | chick69 |
| insecticide1 | low        | sprayed   | week1 | strip3 | swath6 | pen12 | chick70 |
| insecticide1 | low        | sprayed   | week1 | strip3 | swath6 | pen12 | chick71 |

| insecticide  | dose_level | food_type | week  | strip  | swath   | pen   | chick    |
|--------------|------------|-----------|-------|--------|---------|-------|----------|
| insecticide1 | low        | sprayed   | week1 | strip3 | swath6  | pen12 | chick72  |
| insecticide3 | low        | unsprayed | week2 | strip4 | swath7  | pen13 | chick73  |
| insecticide3 | low        | unsprayed | week2 | strip4 | swath7  | pen13 | chick74  |
| insecticide3 | low        | unsprayed | week2 | strip4 | swath7  | pen13 | chick75  |
| insecticide3 | low        | unsprayed | week2 | strip4 | swath7  | pen13 | chick76  |
| insecticide3 | low        | unsprayed | week2 | strip4 | swath7  | pen13 | chick77  |
| insecticide3 | low        | unsprayed | week2 | strip4 | swath7  | pen13 | chick78  |
| insecticide3 | low        | sprayed   | week2 | strip4 | swath7  | pen14 | chick79  |
| insecticide3 | low        | sprayed   | week2 | strip4 | swath7  | pen14 | chick80  |
| insecticide3 | low        | sprayed   | week2 | strip4 | swath7  | pen14 | chick81  |
| insecticide3 | low        | sprayed   | week2 | strip4 | swath7  | pen14 | chick82  |
| insecticide3 | low        | sprayed   | week2 | strip4 | swath7  | pen14 | chick83  |
| insecticide3 | low        | sprayed   | week2 | strip4 | swath7  | pen14 | chick84  |
| insecticide3 | high       | sprayed   | week2 | strip4 | swath8  | pen15 | chick85  |
| insecticide3 | high       | sprayed   | week2 | strip4 | swath8  | pen15 | chick86  |
| insecticide3 | high       | sprayed   | week2 | strip4 | swath8  | pen15 | chick87  |
| insecticide3 | high       | sprayed   | week2 | strip4 | swath8  | pen15 | chick88  |
| insecticide3 | high       | sprayed   | week2 | strip4 | swath8  | pen15 | chick89  |
| insecticide3 | high       | sprayed   | week2 | strip4 | swath8  | pen15 | chick90  |
| insecticide3 | high       | unsprayed | week2 | strip4 | swath8  | pen16 | chick91  |
| insecticide3 | high       | unsprayed | week2 | strip4 | swath8  | pen16 | chick92  |
| insecticide3 | high       | unsprayed | week2 | strip4 | swath8  | pen16 | chick93  |
| insecticide3 | high       | unsprayed | week2 | strip4 | swath8  | pen16 | chick94  |
| insecticide3 | high       | unsprayed | week2 | strip4 | swath8  | pen16 | chick95  |
| insecticide3 | high       | unsprayed | week2 | strip4 | swath8  | pen16 | chick96  |
| insecticide1 | high       | sprayed   | week2 | strip5 | swath9  | pen17 | chick97  |
| insecticide1 | high       | sprayed   | week2 | strip5 | swath9  | pen17 | chick98  |
| insecticide1 | high       | sprayed   | week2 | strip5 | swath9  | pen17 | chick99  |
| insecticide1 | high       | sprayed   | week2 | strip5 | swath9  | pen17 | chick100 |
| insecticide1 | high       | sprayed   | week2 | strip5 | swath9  | pen17 | chick101 |
| insecticide1 | high       | sprayed   | week2 | strip5 | swath9  | pen17 | chick102 |
| insecticide1 | high       | unsprayed | week2 | strip5 | swath9  | pen18 | chick103 |
| insecticide1 | high       | unsprayed | week2 | strip5 | swath9  | pen18 | chick104 |
| insecticide1 | high       | unsprayed | week2 | strip5 | swath9  | pen18 | chick105 |
| insecticide1 | high       | unsprayed | week2 | strip5 | swath9  | pen18 | chick106 |
| insecticide1 | high       | unsprayed | week2 | strip5 | swath9  | pen18 | chick107 |
| insecticide1 | high       | unsprayed | week2 | strip5 | swath9  | pen18 | chick108 |
| insecticide1 | low        | unsprayed | week2 | strip5 | swath10 | pen19 | chick109 |
| insecticide1 | low        | unsprayed | week2 | strip5 | swath10 | pen19 | chick110 |
| insecticide1 | low        | unsprayed | week2 | strip5 | swath10 | pen19 | chick111 |
| insecticide1 | low        | unsprayed | week2 | strip5 | swath10 | pen19 | chick112 |

| insecticide  | dose_level | food_type | week  | strip  | swath   | pen   | chick    |
|--------------|------------|-----------|-------|--------|---------|-------|----------|
| insecticide1 | low        | unsprayed | week2 | strip5 | swath10 | pen19 | chick113 |
| insecticide1 | low        | unsprayed | week2 | strip5 | swath10 | pen19 | chick114 |
| insecticide1 | low        | sprayed   | week2 | strip5 | swath10 | pen20 | chick115 |
| insecticide1 | low        | sprayed   | week2 | strip5 | swath10 | pen20 | chick116 |
| insecticide1 | low        | sprayed   | week2 | strip5 | swath10 | pen20 | chick117 |
| insecticide1 | low        | sprayed   | week2 | strip5 | swath10 | pen20 | chick118 |
| insecticide1 | low        | sprayed   | week2 | strip5 | swath10 | pen20 | chick119 |
| insecticide1 | low        | sprayed   | week2 | strip5 | swath10 | pen20 | chick120 |
| insecticide2 | low        | unsprayed | week2 | strip6 | swath11 | pen21 | chick121 |
| insecticide2 | low        | unsprayed | week2 | strip6 | swath11 | pen21 | chick122 |
| insecticide2 | low        | unsprayed | week2 | strip6 | swath11 | pen21 | chick123 |
| insecticide2 | low        | unsprayed | week2 | strip6 | swath11 | pen21 | chick124 |
| insecticide2 | low        | unsprayed | week2 | strip6 | swath11 | pen21 | chick125 |
| insecticide2 | low        | unsprayed | week2 | strip6 | swath11 | pen21 | chick126 |
| insecticide2 | low        | sprayed   | week2 | strip6 | swath11 | pen22 | chick127 |
| insecticide2 | low        | sprayed   | week2 | strip6 | swath11 | pen22 | chick128 |
| insecticide2 | low        | sprayed   | week2 | strip6 | swath11 | pen22 | chick129 |
| insecticide2 | low        | sprayed   | week2 | strip6 | swath11 | pen22 | chick130 |
| insecticide2 | low        | sprayed   | week2 | strip6 | swath11 | pen22 | chick131 |
| insecticide2 | low        | sprayed   | week2 | strip6 | swath11 | pen22 | chick132 |
| insecticide2 | high       | sprayed   | week2 | strip6 | swath12 | pen23 | chick133 |
| insecticide2 | high       | sprayed   | week2 | strip6 | swath12 | pen23 | chick134 |
| insecticide2 | high       | sprayed   | week2 | strip6 | swath12 | pen23 | chick135 |
| insecticide2 | high       | sprayed   | week2 | strip6 | swath12 | pen23 | chick136 |
| insecticide2 | high       | sprayed   | week2 | strip6 | swath12 | pen23 | chick137 |
| insecticide2 | high       | sprayed   | week2 | strip6 | swath12 | pen23 | chick138 |
| insecticide2 | high       | unsprayed | week2 | strip6 | swath12 | pen24 | chick139 |
| insecticide2 | high       | unsprayed | week2 | strip6 | swath12 | pen24 | chick140 |
| insecticide2 | high       | unsprayed | week2 | strip6 | swath12 | pen24 | chick141 |
| insecticide2 | high       | unsprayed | week2 | strip6 | swath12 | pen24 | chick142 |
| insecticide2 | high       | unsprayed | week2 | strip6 | swath12 | pen24 | chick143 |
| insecticide2 | high       | unsprayed | week2 | strip6 | swath12 | pen24 | chick144 |
| insecticide3 | high       | unsprayed | week3 | strip7 | swath13 | pen25 | chick145 |
| insecticide3 | high       | unsprayed | week3 | strip7 | swath13 | pen25 | chick146 |
| insecticide3 | high       | unsprayed | week3 | strip7 | swath13 | pen25 | chick147 |
| insecticide3 | high       | unsprayed | week3 | strip7 | swath13 | pen25 | chick148 |
| insecticide3 | high       | unsprayed | week3 | strip7 | swath13 | pen25 | chick149 |
| insecticide3 | high       | unsprayed | week3 | strip7 | swath13 | pen25 | chick150 |
| insecticide3 | high       | sprayed   | week3 | strip7 | swath13 | pen26 | chick151 |
| insecticide3 | high       | sprayed   | week3 | strip7 | swath13 | pen26 | chick152 |
| insecticide3 | high       | sprayed   | week3 | strip7 | swath13 | pen26 | chick153 |

| insecticide  | dose_level | food_type | week  | strip  | swath   | pen   | chick    |
|--------------|------------|-----------|-------|--------|---------|-------|----------|
| insecticide3 | high       | sprayed   | week3 | strip7 | swath13 | pen26 | chick154 |
| insecticide3 | high       | sprayed   | week3 | strip7 | swath13 | pen26 | chick155 |
| insecticide3 | high       | sprayed   | week3 | strip7 | swath13 | pen26 | chick156 |
| insecticide3 | low        | unsprayed | week3 | strip7 | swath14 | pen27 | chick157 |
| insecticide3 | low        | unsprayed | week3 | strip7 | swath14 | pen27 | chick158 |
| insecticide3 | low        | unsprayed | week3 | strip7 | swath14 | pen27 | chick159 |
| insecticide3 | low        | unsprayed | week3 | strip7 | swath14 | pen27 | chick160 |
| insecticide3 | low        | unsprayed | week3 | strip7 | swath14 | pen27 | chick161 |
| insecticide3 | low        | unsprayed | week3 | strip7 | swath14 | pen27 | chick162 |
| insecticide3 | low        | sprayed   | week3 | strip7 | swath14 | pen28 | chick163 |
| insecticide3 | low        | sprayed   | week3 | strip7 | swath14 | pen28 | chick164 |
| insecticide3 | low        | sprayed   | week3 | strip7 | swath14 | pen28 | chick165 |
| insecticide3 | low        | sprayed   | week3 | strip7 | swath14 | pen28 | chick166 |
| insecticide3 | low        | sprayed   | week3 | strip7 | swath14 | pen28 | chick167 |
| insecticide3 | low        | sprayed   | week3 | strip7 | swath14 | pen28 | chick168 |
| insecticide2 | low        | unsprayed | week3 | strip8 | swath15 | pen29 | chick169 |
| insecticide2 | low        | unsprayed | week3 | strip8 | swath15 | pen29 | chick170 |
| insecticide2 | low        | unsprayed | week3 | strip8 | swath15 | pen29 | chick171 |
| insecticide2 | low        | unsprayed | week3 | strip8 | swath15 | pen29 | chick172 |
| insecticide2 | low        | unsprayed | week3 | strip8 | swath15 | pen29 | chick173 |
| insecticide2 | low        | unsprayed | week3 | strip8 | swath15 | pen29 | chick174 |
| insecticide2 | low        | sprayed   | week3 | strip8 | swath15 | pen30 | chick175 |
| insecticide2 | low        | sprayed   | week3 | strip8 | swath15 | pen30 | chick176 |
| insecticide2 | low        | sprayed   | week3 | strip8 | swath15 | pen30 | chick177 |
| insecticide2 | low        | sprayed   | week3 | strip8 | swath15 | pen30 | chick178 |
| insecticide2 | low        | sprayed   | week3 | strip8 | swath15 | pen30 | chick179 |
| insecticide2 | low        | sprayed   | week3 | strip8 | swath15 | pen30 | chick180 |
| insecticide2 | high       | sprayed   | week3 | strip8 | swath16 | pen31 | chick181 |
| insecticide2 | high       | sprayed   | week3 | strip8 | swath16 | pen31 | chick182 |
| insecticide2 | high       | sprayed   | week3 | strip8 | swath16 | pen31 | chick183 |
| insecticide2 | high       | sprayed   | week3 | strip8 | swath16 | pen31 | chick184 |
| insecticide2 | high       | sprayed   | week3 | strip8 | swath16 | pen31 | chick185 |
| insecticide2 | high       | sprayed   | week3 | strip8 | swath16 | pen31 | chick186 |
| insecticide2 | high       | unsprayed | week3 | strip8 | swath16 | pen32 | chick187 |
| insecticide2 | high       | unsprayed | week3 | strip8 | swath16 | pen32 | chick188 |
| insecticide2 | high       | unsprayed | week3 | strip8 | swath16 | pen32 | chick189 |
| insecticide2 | high       | unsprayed | week3 | strip8 | swath16 | pen32 | chick190 |
| insecticide2 | high       | unsprayed | week3 | strip8 | swath16 | pen32 | chick191 |
| insecticide2 | high       | unsprayed | week3 | strip8 | swath16 | pen32 | chick192 |
| insecticide1 | high       | sprayed   | week3 | strip9 | swath17 | pen33 | chick193 |
| insecticide1 | high       | sprayed   | week3 | strip9 | swath17 | pen33 | chick194 |

| insecticide  | dose_level | food_type | week  | strip  | swath   | pen   | chick    |
|--------------|------------|-----------|-------|--------|---------|-------|----------|
| insecticide1 | high       | sprayed   | week3 | strip9 | swath17 | pen33 | chick195 |
| insecticide1 | high       | sprayed   | week3 | strip9 | swath17 | pen33 | chick196 |
| insecticide1 | high       | sprayed   | week3 | strip9 | swath17 | pen33 | chick197 |
| insecticide1 | high       | sprayed   | week3 | strip9 | swath17 | pen33 | chick198 |
| insecticide1 | high       | unsprayed | week3 | strip9 | swath17 | pen34 | chick199 |
| insecticide1 | high       | unsprayed | week3 | strip9 | swath17 | pen34 | chick200 |
| insecticide1 | high       | unsprayed | week3 | strip9 | swath17 | pen34 | chick201 |
| insecticide1 | high       | unsprayed | week3 | strip9 | swath17 | pen34 | chick202 |
| insecticide1 | high       | unsprayed | week3 | strip9 | swath17 | pen34 | chick203 |
| insecticide1 | high       | unsprayed | week3 | strip9 | swath17 | pen34 | chick204 |
| insecticide1 | low        | sprayed   | week3 | strip9 | swath18 | pen35 | chick205 |
| insecticide1 | low        | sprayed   | week3 | strip9 | swath18 | pen35 | chick206 |
| insecticide1 | low        | sprayed   | week3 | strip9 | swath18 | pen35 | chick207 |
| insecticide1 | low        | sprayed   | week3 | strip9 | swath18 | pen35 | chick208 |
| insecticide1 | low        | sprayed   | week3 | strip9 | swath18 | pen35 | chick209 |
| insecticide1 | low        | sprayed   | week3 | strip9 | swath18 | pen35 | chick210 |
| insecticide1 | low        | unsprayed | week3 | strip9 | swath18 | pen36 | chick211 |
| insecticide1 | low        | unsprayed | week3 | strip9 | swath18 | pen36 | chick212 |
| insecticide1 | low        | unsprayed | week3 | strip9 | swath18 | pen36 | chick213 |
| insecticide1 | low        | unsprayed | week3 | strip9 | swath18 | pen36 | chick214 |
| insecticide1 | low        | unsprayed | week3 | strip9 | swath18 | pen36 | chick215 |
| insecticide1 | low        | unsprayed | week3 | strip9 | swath18 | pen36 | chick216 |

## Unbalanced Factorial Design

Here we consider the first four motion sickness experiments reported in Burns (1984).

```

1  des3 <- design("Motion sickness incidence") %>%
2    set_units(experiment = 4,
3              subject = nested_in(experiment,
4                                  1 ~ 21,
5                                  2 ~ 20,
6                                  3 ~ 29,
7                                  4 ~ 59)) %>%
8    set_trts(frequency = c(0.167, 0.250),
9             acceleration = c(0.111, 0.222)) %>%
10   allot_trts(frequency:acceleration ~ experiment) %>%
11   assign_trts(order = "systematic") %>%
12   serve_table()

```

Table 3: Design table output for the unbalanced factorial design.

| experiment  | subject   | frequency | acceleration |
|-------------|-----------|-----------|--------------|
| experiment1 | subject1  | 0.167     | 0.111        |
| experiment1 | subject2  | 0.167     | 0.111        |
| experiment1 | subject3  | 0.167     | 0.111        |
| experiment1 | subject4  | 0.167     | 0.111        |
| experiment1 | subject5  | 0.167     | 0.111        |
| experiment1 | subject6  | 0.167     | 0.111        |
| experiment1 | subject7  | 0.167     | 0.111        |
| experiment1 | subject8  | 0.167     | 0.111        |
| experiment1 | subject9  | 0.167     | 0.111        |
| experiment1 | subject10 | 0.167     | 0.111        |
| experiment1 | subject11 | 0.167     | 0.111        |
| experiment1 | subject12 | 0.167     | 0.111        |
| experiment1 | subject13 | 0.167     | 0.111        |
| experiment1 | subject14 | 0.167     | 0.111        |
| experiment1 | subject15 | 0.167     | 0.111        |
| experiment1 | subject16 | 0.167     | 0.111        |
| experiment1 | subject17 | 0.167     | 0.111        |
| experiment1 | subject18 | 0.167     | 0.111        |
| experiment1 | subject19 | 0.167     | 0.111        |
| experiment1 | subject20 | 0.167     | 0.111        |
| experiment1 | subject21 | 0.167     | 0.111        |
| experiment2 | subject22 | 0.25      | 0.111        |
| experiment2 | subject23 | 0.25      | 0.111        |
| experiment2 | subject24 | 0.25      | 0.111        |
| experiment2 | subject25 | 0.25      | 0.111        |
| experiment2 | subject26 | 0.25      | 0.111        |
| experiment2 | subject27 | 0.25      | 0.111        |
| experiment2 | subject28 | 0.25      | 0.111        |
| experiment2 | subject29 | 0.25      | 0.111        |
| experiment2 | subject30 | 0.25      | 0.111        |
| experiment2 | subject31 | 0.25      | 0.111        |
| experiment2 | subject32 | 0.25      | 0.111        |
| experiment2 | subject33 | 0.25      | 0.111        |
| experiment2 | subject34 | 0.25      | 0.111        |
| experiment2 | subject35 | 0.25      | 0.111        |
| experiment2 | subject36 | 0.25      | 0.111        |
| experiment2 | subject37 | 0.25      | 0.111        |
| experiment2 | subject38 | 0.25      | 0.111        |
| experiment2 | subject39 | 0.25      | 0.111        |

| experiment  | subject   | frequency | acceleration |
|-------------|-----------|-----------|--------------|
| experiment2 | subject40 | 0.25      | 0.111        |
| experiment2 | subject41 | 0.25      | 0.111        |
| experiment3 | subject42 | 0.167     | 0.222        |
| experiment3 | subject43 | 0.167     | 0.222        |
| experiment3 | subject44 | 0.167     | 0.222        |
| experiment3 | subject45 | 0.167     | 0.222        |
| experiment3 | subject46 | 0.167     | 0.222        |
| experiment3 | subject47 | 0.167     | 0.222        |
| experiment3 | subject48 | 0.167     | 0.222        |
| experiment3 | subject49 | 0.167     | 0.222        |
| experiment3 | subject50 | 0.167     | 0.222        |
| experiment3 | subject51 | 0.167     | 0.222        |
| experiment3 | subject52 | 0.167     | 0.222        |
| experiment3 | subject53 | 0.167     | 0.222        |
| experiment3 | subject54 | 0.167     | 0.222        |
| experiment3 | subject55 | 0.167     | 0.222        |
| experiment3 | subject56 | 0.167     | 0.222        |
| experiment3 | subject57 | 0.167     | 0.222        |
| experiment3 | subject58 | 0.167     | 0.222        |
| experiment3 | subject59 | 0.167     | 0.222        |
| experiment3 | subject60 | 0.167     | 0.222        |
| experiment3 | subject61 | 0.167     | 0.222        |
| experiment3 | subject62 | 0.167     | 0.222        |
| experiment3 | subject63 | 0.167     | 0.222        |
| experiment3 | subject64 | 0.167     | 0.222        |
| experiment3 | subject65 | 0.167     | 0.222        |
| experiment3 | subject66 | 0.167     | 0.222        |
| experiment3 | subject67 | 0.167     | 0.222        |
| experiment3 | subject68 | 0.167     | 0.222        |
| experiment3 | subject69 | 0.167     | 0.222        |
| experiment3 | subject70 | 0.167     | 0.222        |
| experiment4 | subject71 | 0.25      | 0.222        |
| experiment4 | subject72 | 0.25      | 0.222        |
| experiment4 | subject73 | 0.25      | 0.222        |
| experiment4 | subject74 | 0.25      | 0.222        |
| experiment4 | subject75 | 0.25      | 0.222        |
| experiment4 | subject76 | 0.25      | 0.222        |
| experiment4 | subject77 | 0.25      | 0.222        |
| experiment4 | subject78 | 0.25      | 0.222        |
| experiment4 | subject79 | 0.25      | 0.222        |
| experiment4 | subject80 | 0.25      | 0.222        |

| experiment  | subject    | frequency | acceleration |
|-------------|------------|-----------|--------------|
| experiment4 | subject81  | 0.25      | 0.222        |
| experiment4 | subject82  | 0.25      | 0.222        |
| experiment4 | subject83  | 0.25      | 0.222        |
| experiment4 | subject84  | 0.25      | 0.222        |
| experiment4 | subject85  | 0.25      | 0.222        |
| experiment4 | subject86  | 0.25      | 0.222        |
| experiment4 | subject87  | 0.25      | 0.222        |
| experiment4 | subject88  | 0.25      | 0.222        |
| experiment4 | subject89  | 0.25      | 0.222        |
| experiment4 | subject90  | 0.25      | 0.222        |
| experiment4 | subject91  | 0.25      | 0.222        |
| experiment4 | subject92  | 0.25      | 0.222        |
| experiment4 | subject93  | 0.25      | 0.222        |
| experiment4 | subject94  | 0.25      | 0.222        |
| experiment4 | subject95  | 0.25      | 0.222        |
| experiment4 | subject96  | 0.25      | 0.222        |
| experiment4 | subject97  | 0.25      | 0.222        |
| experiment4 | subject98  | 0.25      | 0.222        |
| experiment4 | subject99  | 0.25      | 0.222        |
| experiment4 | subject100 | 0.25      | 0.222        |
| experiment4 | subject101 | 0.25      | 0.222        |
| experiment4 | subject102 | 0.25      | 0.222        |
| experiment4 | subject103 | 0.25      | 0.222        |
| experiment4 | subject104 | 0.25      | 0.222        |
| experiment4 | subject105 | 0.25      | 0.222        |
| experiment4 | subject106 | 0.25      | 0.222        |
| experiment4 | subject107 | 0.25      | 0.222        |
| experiment4 | subject108 | 0.25      | 0.222        |
| experiment4 | subject109 | 0.25      | 0.222        |
| experiment4 | subject110 | 0.25      | 0.222        |
| experiment4 | subject111 | 0.25      | 0.222        |
| experiment4 | subject112 | 0.25      | 0.222        |
| experiment4 | subject113 | 0.25      | 0.222        |
| experiment4 | subject114 | 0.25      | 0.222        |
| experiment4 | subject115 | 0.25      | 0.222        |
| experiment4 | subject116 | 0.25      | 0.222        |
| experiment4 | subject117 | 0.25      | 0.222        |
| experiment4 | subject118 | 0.25      | 0.222        |
| experiment4 | subject119 | 0.25      | 0.222        |
| experiment4 | subject120 | 0.25      | 0.222        |
| experiment4 | subject121 | 0.25      | 0.222        |

| experiment  | subject    | frequency | acceleration |
|-------------|------------|-----------|--------------|
| experiment4 | subject122 | 0.25      | 0.222        |
| experiment4 | subject123 | 0.25      | 0.222        |
| experiment4 | subject124 | 0.25      | 0.222        |
| experiment4 | subject125 | 0.25      | 0.222        |
| experiment4 | subject126 | 0.25      | 0.222        |
| experiment4 | subject127 | 0.25      | 0.222        |
| experiment4 | subject128 | 0.25      | 0.222        |
| experiment4 | subject129 | 0.25      | 0.222        |

## Acknowledgement

This paper uses `knitr` (Xie 2015), `rmarkdown` (Xie, Allaire, and Golemund 2018) and Quarto for creating reproducible documents. The code presented uses version 0.1.3 of the `edibble` package available on CRAN. The latest development of `edibble` can be found at <https://github.com/emitanaka/edibble>.

## References

- Burns, K. C. 1984. “[Motion Sickness Incidence: Distribution of Time to First Emesis and Comparison of Some Complex Motion Conditions.](#)” *Aviation, Space, and Environmental Medicine* 55 (6): 521–27.
- Fisher, Ronald A. 1950. *Statistical Methods for Research Workers*. 11th ed. Oliver and Boyd.
- Martin, Pamela A., Daniel L. Johnson, and Douglas J. Forsyth. 1996. “Effects of Grasshopper-Control Insecticides on Survival and Brain Acetylcholinesterase of Pheasant ( *Phasianus Colchicus* ) Chicks.” *Environmental Toxicology and Chemistry / SETAC* 15 (4): 518–24. [https://doi.org/10.1897/1551-5028\(1996\)015%3C0518:EOGCIO%3E2.3.CO;2](https://doi.org/10.1897/1551-5028(1996)015%3C0518:EOGCIO%3E2.3.CO;2).
- R Core Team. 2020. *R: A Language and Environment for Statistical Computing*. Vienna, Austria: R Foundation for Statistical Computing. <https://www.R-project.org/>.
- Tanaka, Emi. 2023. *edibble: Designing Comparative Experiments*. <https://CRAN.R-project.org/package=edibble>.
- Xie, Yihui. 2015. *Dynamic Documents with R and Knitr*. 2nd ed. Boca Raton, Florida: Chapman; Hall/CRC. <https://yihui.org/knitr/>.
- Xie, Yihui, J. J. Allaire, and Garrett Golemund. 2018. *R Markdown: The Definitive Guide*. Boca Raton, Florida: Chapman; Hall/CRC. <https://bookdown.org/yihui/rmarkdown>.
